# Supplementary material for: Online Set-Based Dynamic Analysis for Sound Predictive Race Detection
Source: arXiv:1907.08337 source file (2019-07-19)
Supplement: Supplementary file 1 [file Appendix-Examples.tex]

%auto-ignore
\section{Example Executions Analyzed by \GoldCP}
\label{sec:appendix-examples}

\mike{Haven't read this yet since I don't know if it's ready or what's the plan for it,
\eg, the figures at least don't use the new format for analysis state updates,
which is potentially okay, especially if you think the new format wouldn't fit.}
\jake{To start off, there are 5 figures representing 6 examples and
among those 6 only 4 examples are unique (not reused for a different
explination) and 2 of the 4 are different by a single event (read(y) vs.
read(z)). The following is a list of the figures and my throughts on them to be
used as comparison or guideline to determining if the appendix examples should
be included and why:
\begin{itemize}
  \item Figure 1 has two examples differed by the variable being read
  demonstrating the difference between CP-race and not a CP-race. Important
  fundamental to undestanding predictive analysis. Figure and both examples are
  needed.
  \item Figure 2 has a new example to demonstrate the delayed informaion needed
  to correctly establish order and detect a race. The figure itself
  represents how ordering is establish at each event. Figure and example are
  needed.
  \item Figure 4 (Figure 3 is the invariants) reuses the example in Figure 1(b).
  The figure itself shows the elements added and removed at every event for all
  set owners. Using a common example means the reader can be relied on to
  understand the example on a basic level allowing the new elements to take
  focus. Figure is needed and, though Figure 1(a) or Figure 2 could work,
  Figure 1(b) example is a good choice.
  \item Figure 5 reuses the example in Figure 2 to demonstrate the same element
  add and remove as Figure 4 with a more complex example that has already been
  introduced. The figure is useful to show how an added element translates to an
  ordering being established by comparing Figure 4 and Figure 2. Figure is not
  needed but is a useful guide to understanding the relationship
  between the algorithm and the relation as well as a further explination of an
  already complex example. I would argue an example like this needs to exist
  but this specific example is not needed.
  \item Figure 6 is a new example to demonstrate the transfer of CCP elements,
  similar to Figure 4 and 5's element add and remove. This figure is needed to
  show how CCP elements are transferred, arguably the most difficult concept to
  understand of the algorithm.
\end{itemize}
Based on these examples the remaining examples in the appendix will be judged on
usefulness to the already established examples in the main paper.}

% This section shows additional examples that are more complex than the example
% in Figure~\ref{fig:simple-analysis-example} from Section~\ref{Sec:analysis:examples}.

\subsection{Example Involving \CP Ordering Established Before Accesses Execute}
% \paragraph{Example involving \CP ordering established before accesses execute.}

\jake{This example and the next one are not showing anything more than Figure
5 but are more complex example. I think Figure 2 and 5 (same example) are better
for explaining the concepts earlier in the paper. The advantage of this example and
the next one is to show the subtle difference between the two traces. My
suggestion is to change Figure 5 so that the critical section on m by T1
executes before the access to x by T1 to show this subtle difference. That would
cut down on introducing new examples while allowing the subtle difference point
to be made.
\mike{Hmm, I like that Figures 2 and 5 are the same example, not slightly different from each other
(which would make it harder for the reader to see how \raptor manages the knowable info at each step).}}

\begin{figure}
\smaller
\centering

\newcolumntype{L}{>{$}l<{$}} % math-mode version of "l" column type

\begin{tabular}{@{}l@{\;}l@{\;\;}l@{\;}l@{\;}|L@{}}
\thr{T1} & \thr{T2} & \thr{T3} & \thr{T4} & \text{Updated analysis state after event (excluding \POLockSetPlain{\rho}{})}\\\hline
&\Acquire{m}{1}&&& \HBLockSet{m}{1} = \{\HBThread{T2}\}\\
&\Acquire{q}{1}&&& \HBLockSet{q}{1} = \{\HBThread{T2}\}\\
&\Release{q}{1}&&& \HBLockSet{m}{1} = \HBLockSet{q}{1} = \{\HBLock{q}{1}, \HBThread{T2}\}\\
&&\Acquire{q}{2}&& \HBLockSet{q}{2} = \{\HBThread{T3}\}, \HBLockSet{m}{1} = \HBLockSet{q}{1} = \{\HBLock{q}{1}, \HBThread{T2}, \HBThread{T3}\}, \PCPLockSet{m}{1} = \PCPLockSet{q}{1} = \{\PCPThread{T3}{q}{1}\}\\
&&\Release{q}{2}&& \HBLockSet{q}{2} = \{\HBLock{q}{2}, \HBThread{T3}\}, \CCPLockSet{m}{1} = \CCPLockSet{q}{1} = \emptyset\\
&&\Acquire{n}{1}&& \HBLockSet{n}{1} = \{\HBThread{T3}\}\\
&&\Write{y}{1}&& \HBLockSet{y}{1} = \{\LSLock{n}{1}, \HBThread{T3}\}\\
&&\Release{n}{1}\tikzmark{1}&& \HBLockSet{q}{2} = \{\HBLock{q}{2}, \HBLock{n}{1}, \HBThread{T3}\}, \HBLockSet{n}{1} = \{\HBLock{n}{1}, \HBThread{T3}\}, \HBLockSet{m}{1} = \HBLockSet{q}{1} = \{\HBLock{q}{1}, \HBLock{n}{1}, \HBThread{T2}, \HBThread{T3}\}\\
&&&\tikzmark{2}\Acquire{n}{2}& \HBLockSet{y}{1} = \{\LSLock{n}{1}, \HBThread{T3}, \HBThread{T4}\}, \HBLockSet{q}{2} = \{\HBLock{q}{2}, \HBLock{n}{1}, \HBThread{T3}, \HBThread{T4}\}, \HBLockSet{n}{1} = \{\HBLock{n}{1}, \HBThread{T3}, \HBThread{T4}\},\\
&&&& \HBLockSet{m}{1} = \HBLockSet{q}{1} = \{\HBLock{q}{1}, \HBLock{n}{1}, \HBThread{T2}, \HBThread{T3}, \HBThread{T4}\}, \HBLockSet{n}{2} = \{\HBThread{T4}\},\\
&&&& \PCPLockSet{m}{1} = \PCPLockSet{q}{1} = \PCPLockSet{q}{2} = \PCPLockSet{n}{1} = \PCPLockSet{y}{1} = \{\PCPThread{T4}{n}{1}\}\\
&&&\Write{y}{2}& \HBLockSet{y}{1} = \{\LSLock{n}{1}, \HBThread{T3}, \HBThread{T4}, \HBThreadPlain{\xi}\}, \HBLockSet{y}{2} = \{\LSLock{n}{2}, \HBThread{T4}\}, \CPLockSet{n}{1} = \{\CPThread{T4}\}, \PCPLockSet{y}{1} = \{\PCPThread{T4}{n}{1}, \PCPThread{$\xi$}{n}{1}\}\\
&&&\Release{n}{2}& \HBLockSet{n}{2} = \{\HBLock{n}{2}, \HBThread{T4}\}, \CPLockSet{y}{1} = \{\CPLock{n}, \CPThread{T4}, \CPThread{$\xi$}\}, \CPLockSet{m}{1} = \CPLockSet{q}{1} = \CPLockSet{q}{2} = \CPLockSet{n}{1} = \{\CPLock{n}, \CPThread{T4}\},\\
&&&& \PCPLockSet{m}{1} = \PCPLockSet{q}{1} = \PCPLockSet{q}{2} = \PCPLockSet{n}{1} = \PCPLockSet{y}{1} = \emptyset\\
\Write{x}{1}&&&& \HBLockSet{x}{1} = \{\HBThread{T1}\}\\
\Acquire{p}{1}&&&& \HBLockSet{p}{1} = \{\HBThread{T1}\}\\
\Release{p}{1}&&&& \HBLockSet{p}{1} = \HBLockSet{x}{1} = \{\HBLock{p}{1}, \HBThread{T1}\},\\
&\Acquire{p}{2}&&& \HBLockSet{p}{1} = \HBLockSet{x}{1} = \{\HBLock{p}{1}, \HBThread{T1}, \HBThread{T2}\}, \HBLockSet{p}{2} = \{\HBThread{T2}\}, \PCPLockSet{p}{1} = \PCPLockSet{x}{1} = \{\PCPThread{T2}{p}{1}\}\\
&\Release{p}{2}&&& \HBLockSet{m}{1} = \HBLockSet{q}{1} = \{\HBLock{q}{1}, \HBLock{n}{1}, \HBLock{p}{2}, \HBThread{T2}, \HBThread{T3}, \HBThread{T4}\}, \HBLockSet{p}{2} = \{\HBLock{p}{2}, \HBThread{T2}\},\\
&&&& \CCPLockSet{p}{1} = \CCPLockSet{x}{1} = \emptyset\\
&\Release{m}{1}&&& \HBLockSet{p}{1} = \HBLockSet{x}{1} = \{\HBLock{p}{1}, \HBLock{m}{1}, \HBThread{T1}, \HBThread{T2}\}, \HBLockSet{m}{1} = \HBLockSet{q}{1} = \{\HBLock{q}{1}, \HBLock{n}{1}, \HBLock{p}{2}, \HBLock{m}{1}, \HBThread{T2}, \HBThread{T3}, \HBThread{T4}\}\\
&&&& \HBLockSet{p}{2} = \{\HBLock{p}{2}, \HBLock{m}{1}, \HBThread{T2}\}\\
&&&\Acquire{m}{2}& \HBLockSet{p}{1} = \HBLockSet{x}{1} = \{\HBLock{p}{1}, \HBLock{m}{1}, \HBThread{T1}, \HBThread{T2}, \HBThread{T4}\}, \HBLockSet{p}{2} = \{\HBLock{p}{2}, \HBLock{m}{1}, \HBThread{T2}, \HBThread{T4}\}, \HBLockSet{m}{2} = \{\HBThread{T4}\}\\
&&&& \PCPLockSet{p}{1} = \PCPLockSet{p}{2} = \PCPLockSet{x}{1} = \PCPLockSet{m}{1} = \PCPLockSet{q}{1} = \{\PCPThread{T4}{m}{1}\}\\
&&&\Release{m}{2}& \HBLockSet{m}{2} = \{\HBLock{m}{2}, \HBThread{T4}\}, \HBLockSet{n}{2} = \{\HBLock{n}{2}, \HBLock{m}{2}, \HBThread{T4}\}, \HBLockSet{y}{1} = \{\LSLock{n}{1}, \HBLock{m}{2}, \HBThread{T3}, \HBThread{T4}, \HBThreadPlain{\xi}\},\\
&&&& \HBLockSet{q}{2} = \{\HBLock{q}{2}, \HBLock{n}{1}, \HBLock{m}{2}, \HBThread{T3}, \HBThread{T4}\}, \HBLockSet{y}{2} = \{\LSLock{n}{2}, \HBLock{m}{2}, \HBThread{T4}\}, \HBLockSet{n}{1} = \{\HBLock{n}{1}, \HBLock{m}{2}, \HBThread{T3}, \HBThread{T4}\},\\
&&&& \CPLockSet{p}{1} = \CPLockSet{p}{2} = \CPLockSet{x}{1} = \{\CPLock{m}, \CPThread{T4}\}, \CPLockSet{y}{1} = \{\CPLock{n}, \CPLock{m}, \CPThread{T4}, \CPThread{$\xi$}\},\\
&&&& \CPLockSet{m}{1} = \CPLockSet{q}{1} = \CPLockSet{q}{2} = \CPLockSet{n}{1} = \{\CPLock{n}, \CPLock{m}, \CPThread{T4}\},\\
&&&& \CCPLockSet{p}{1} = \CCPLockSet{p}{2} = \CCPLockSet{x}{1} = \CCPLockSet{m}{1} = \CCPLockSet{q}{1} = \emptyset\\
&&&\Write{x}{2}& \HBLockSet{x}{2} = \{\HBThread{T4}\}, \CPLockSet{x}{1} = \{\CPLock{m}, \CPThread{T4}, \CPThreadPlain{\xi}\}, \HBLockSet{x}{1} = \{\HBLock{p}{1}, \HBLock{m}{1}, \HBThread{T1}, \HBThread{T2}, \HBThread{T4}, \HBThreadPlain{\xi} \}\\

\end{tabular}
\textlink{1}{2}{\CP}

% \mike{Shouldn't \CPLockSet{x}{1} and \HBLockSet{x}{1} contain $\xi$ after \Write{x}{2}?
% \mike{Jake!}}

% \mike{I think all examples should use \thr{T1} etc.\ (since those are in fact lockset elements used by the analysis). I'll make this change.}

\caption{Example execution and \goldCP's analysis state.
\CPOrdered{\Write{x}{1}}{\Write{x}{2}} because \CPOrdered{\Release{n}{1}}{\Acquire{n}{2}}, yet
\Write{x}{1} executes only after \CPOrdered{\Release{n}{1}}{\Acquire{n}{2}} has been established
and after \Release{n}{2} has executed.}
\label{fig:ruleb-late-variable-access}
\end{figure}

Figure~\ref{fig:ruleb-late-variable-access} shows an execution in which both conflicting accesses, \Write{x}{1} and \Write{x}{2},
execute after the initial \CP ordering has been established. The writes to \code{x} are \CP ordered through the following logic:
\CPOrdered{\Release{n}{1}}{\Acquire{n}{2}} by \RuleA implies
% \CPOrdered{\Release{q}{1}}{\Acquire{n}{2}} by \RuleC, which implies
\CPOrdered{\Acquire{m}{1}}{\Release{m}{2}} by \RuleC
(since \HBOrdered{\Acquire{m}{1}}{\Release{n}{1}} and \HBOrdered{\Acquire{n}{2}}{\Release{m}{2}}) implies
\CPOrdered{\Release{m}{1}}{\Acquire{m}{2}} by \RuleB.
% %
Thus
\CPOrdered{\Write{x}{1}}{\Write{x}{2}} by applying \RuleC to
\CPOrdered{\Release{m}{1}}{\Acquire{m}{2}}
(since \HBOrdered{\Write{x}{1}}{\Release{m}{1}} and \HBOrdered{\Acquire{m}{2}}{\Write{x}{2}}).
% through the following logic:
% \HBOrdered{\Write{x}{1}}{\Release{m}{1}} by \HB relation implies
% \CPOrdered{\Write{x}{1}}{\Acquire{m}{2}} by \RuleC implies
% \CPOrdered{\Write{x}{1}}{\Write{x}{2}} by \RuleC.

Since the critical section on \OwnerElement{n}{2} finishes before \Write{x}{1} executes,
\goldCP must keep track of the ordering on critical sections of \code{n}, \code{m}, and other locks---not
just analysis state for variable accesses.
% in addition to analysis state for accesses to \code{x}.
After \Acquire{q}{2}, $\PCPThread{T3}{q}{1} \in \PCPLockSet{m}{1}$.
The \PCP ordering composes with \HB, so that $\PCPThread{T4}{n}{1} \in \PCPLockSet{m}{1}$ before \Release{n}{2},
and thus $\CPThread{T4} \in \CPLockSet{m}{1}$ after \Release{n}{2}.
% This information allows \goldCP to determine \CPOrdered{\Acquire{m}{1}}{\Release{m}{2}}
% and thus \CPOrdered
In a similar vein, \goldCP adds \PCPThread{T4}{m}{1} to \PCPLockSet{x}{1} at \Acquire{m}{2},
which allows the analysis to add \CPThread{T4} to \CPLockSet{x}{1} at \Release{m}{2}.
\notes{\mike{My revised explanation gets more into the weeds than yours (which is commented out below).
But I think that level of detail is useful for helpful the reader understand exactly which steps
and locksets and elements are the important ones for the point(s) we're trying to make.}}%

% The \CP relation established between the conflicting accesses on
% \OwnerElement{x}{} is tracked before the \Write{x}{1}. So the lockset
% owner \Write{x}{1} is unaware of the vital analysis state before its access.
% Even before the access to variable \OwnerElement{y}{}, vital analysis state must
% be collected for lock \HBLock{m}{1} and \HBLock{q}{1}. Therefore, the analysis
% state locks track is just as necessary as the analysis state variables track in
% order to determine \CP relations.

\subsection{Examples that Differ Subtly from Each Other}
% \paragraph{Example involving \CP ordering established only after \CP-ordered variable accesses have executed.}

\begin{figure}
\smaller
\centering

\newcolumntype{L}{>{$}l<{$}} % math-mode version of "l" column type

\begin{tabular}{@{}l@{\;}l@{\;\;}l@{\;}l@{\;}|L@{}}
\thr{T1} & \thr{T2} & \thr{T3} & \thr{T4} & \text{Updated analysis state after event (excluding \POLockSetPlain{\rho}{})}\\\hline
\Write{z}{1}&&&& \HBLockSet{z}{1} = \{\HBThread{T1}\}\\
\Acquire{m}{1}&&&& \HBLockSet{m}{1} = \{\HBThread{T1}\}\\
\Release{m}{1}&&&& \HBLockSet{z}{1} = \HBLockSet{m}{1} = \{\HBLock{m}{1}, \HBThread{T1}\}\\
\Acquire{q}{1}&&&& \HBLockSet{q}{1} = \{\HBThread{T1}\}\\
\Release{q}{1}&&&& \HBLockSet{q}{1} = \{\HBLock{q}{1}, \HBThread{T1}\}, \HBLockSet{z}{1} = \HBLockSet{m}{1} = \{\HBLock{m}{1}, \HBLock{q}{1}, \HBThread{T1}\}\\
&\Acquire{q}{2}&&& \HBLockSet{q}{1} = \{\HBLock{q}{1}, \HBThread{T1}, \HBThread{T2}\}, \HBLockSet{z}{1} = \HBLockSet{m}{1} = \{\HBLock{m}{1}, \HBLock{q}{1}, \HBThread{T1}, \HBThread{T2}\}, \HBLockSet{q}{2} = \{\HBThread{T2}\}\\
&&&& \PCPLockSet{q}{1} = \PCPLockSet{z}{1} = \PCPLockSet{m}{1} = \{\PCPThread{T2}{q}{1}\}\\
&\Release{q}{2}&&& \HBLockSet{q}{2} = \{\HBLock{q}{2}, \HBThread{T2}\}, \PCPLockSet{q}{1} = \PCPLockSet{z}{1} = \PCPLockSet{m}{1} = \emptyset\\
&\Acquire{n}{1}&&& \HBLockSet{n}{1} = \{\HBThread{T2}\}\\
&\Write{y}{1}&&& \HBLockSet{y}{1} = \{\LSLock{n}{1}, \HBThread{T2}\}\\
&\Release{n}{1}\tikzmark{1}&&& \HBLockSet{q}{1} = \{\HBLock{q}{1}, \HBLock{n}{1}, \HBThread{T1}, \HBThread{T2}\}, \HBLockSet{z}{1} = \HBLockSet{m}{1} = \{\HBLock{m}{1}, \HBLock{q}{1}, \HBLock{n}{1}, \HBThread{T1}, \HBThread{T2}\},\\ 
&&&& \HBLockSet{q}{2} = \{\HBLock{q}{2}, \HBLock{n}{1}, \HBThread{T2}\}, \HBLockSet{n}{1} = \{\HBLock{n}{1}, \HBThread{T2}\}\\
&&\Acquire{m}{2}&& \HBLockSet{z}{1} = \HBLockSet{m}{1} = \{\HBLock{m}{1}, \HBLock{q}{1}, \HBLock{n}{1}, \HBThread{T1}, \HBThread{T2}, \HBThread{T3}\}, \HBLockSet{m}{2} = \{\HBThread{T3}\}, \PCPLockSet{z}{1} = \PCPLockSet{m}{1} = \{\PCPThread{T3}{m}{1}\}\\
&&\Acquire{o}{1}&& \HBLockSet{o}{1} = \{\HBThread{T3}\}\\
&&\Release{o}{1}&& \HBLockSet{z}{1} = \HBLockSet{m}{1} = \{\HBLock{m}{1}, \HBLock{q}{1}, \HBLock{n}{1}, \HBLock{o}{1}, \HBThread{T1}, \HBThread{T2}, \HBThread{T3}\}, \HBLockSet{o}{1} = \HBLockSet{m}{2} = \{\HBLock{o}{1}, \HBThread{T3}\}\\
&&&& \PCPLockSet{z}{1} = \PCPLockSet{m}{1} = \{\PCPLock{o}{m}{1}, \PCPThread{T3}{m}{1}\}\\
&&&\Acquire{o}{2}& \HBLockSet{z}{1} = \HBLockSet{m}{1} = \{\HBLock{m}{1}, \HBLock{q}{1}, \HBLock{n}{1}, \HBLock{o}{1}, \HBThread{T1}, \HBThread{T2}, \HBThread{T3}, \HBThread{T4}\}, \HBLockSet{o}{1} = \HBLockSet{m}{2} = \{\HBLock{o}{1}, \HBThread{T3}, \HBThread{T4}\},\\
&&&& \HBLockSet{o}{2} = \{\HBThread{T4}\}, \PCPLockSet{z}{1} = \PCPLockSet{m}{1} = \{\PCPLock{o}{m}{1}, \PCPThread{T4}{m}{1}, \PCPThread{T3}{m}{1}, \PCPThread{T4}{o}{1}\}\\
&&&& \PCPLockSet{o}{1} = \PCPLockSet{m}{1} = \{\PCPThread{T4}{o}{1}\}\\
&&&\Release{o}{2}& \HBLockSet{o}{2} = \{\HBLock{o}{2}, \HBThread{T4}\}, \PCPLockSet{z}{1} = \PCPLockSet{m}{1} = \{\PCPLock{o}{m}{1}, \PCPThread{T4}{m}{1}, \PCPThread{T3}{m}{1}\}, \CCPLockSet{o}{1} = \CCPLockSet{m}{1} = \emptyset\\
&&&\Write{z}{2}& \HBLockSet{z}{2} = \{\HBThread{T4}\}, \HBLockSet{z}{1} = \{\HBLock{m}{1}, \HBLock{q}{1}, \HBLock{n}{1}, \HBLock{o}{1}, \HBThread{T1}, \HBThread{T2}, \HBThread{T3}, \HBThread{T4}, \HBThreadPlain{\xi}\},\\
&&&& \PCPLockSet{z}{1} = \{\PCPLock{o}{m}{1}, \PCPThread{T4}{m}{1}, \PCPThread{T3}{m}{1}, \PCPThread{$\xi$}{m}{1}\}\\
&&\tikzmark{2}\Acquire{n}{2}&& \HBLockSet{q}{1} = \{\HBLock{q}{1}, \HBLock{n}{1}, \HBThread{T1}, \HBThread{T2}, \HBThread{T3}\}, \HBLockSet{q}{2} = \{\HBLock{q}{2}, \HBLock{n}{1}, \HBThread{T2}, \HBThread{T3}\}, \HBLockSet{n}{1} = \{\HBLock{n}{1}, \HBThread{T2}, \HBThread{T3}\},\\
&&&& \HBLockSet{n}{2} = \{\HBThread{T3}\}, \HBLockSet{y}{1} = \{\LSLock{n}{1}, \HBThread{T2}, \HBThread{T3}\}, \PCPLockSet{m}{1} = \{\PCPLock{o}{m}{1}, \PCPThread{T4}{m}{1}, \PCPThread{T3}{m}{1}, \PCPThread{T3}{n}{1}\},\\
&&&& \PCPLockSet{z}{1} = \{\PCPLock{o}{m}{1}, \PCPThread{T4}{m}{1}, \PCPThread{T3}{m}{1}, \PCPThread{$\xi$}{m}{1}, \PCPThread{T3}{n}{1}\},\\
&&&& \PCPLockSet{y}{1} = \PCPLockSet{n}{1} = \PCPLockSet{q}{1} = \PCPLockSet{q}{2} = \{\PCPThread{T3}{n}{1}\}\\
&&\Write{y}{2}&& \HBLockSet{y}{1} = \{\LSLock{n}{1}, \HBThread{T2}, \HBThread{T3}, \HBThreadPlain{\xi}\}, \HBLockSet{y}{2} = \{\LSLock{m}{2}, \LSLock{n}{2}, \HBThread{T3}\}, \CPLockSet{n}{1} = \{\CPThread{T3}\}, \PCPLockSet{y}{1} = \{\PCPThread{T3}{n}{1}, \PCPThreadPlain{\xi}{n}{1}\}\\
&&\Release{n}{2}&& \HBLockSet{o}{1} = \HBLockSet{m}{2} = \{\HBLock{o}{1}, \HBLock{n}{2}, \HBThread{T3}, \HBThread{T4}\}, \HBLockSet{n}{2} = \{\HBLock{n}{2}, \HBThread{T3}\},\\
&&&& \CPLockSet{z}{1} = \CPLockSet{m}{1} = \CPLockSet{n}{1} = \CPLockSet{q}{1} = \CPLockSet{q}{2} = \{\CPLock{n}, \CPThread{T3}\}, \CPLockSet{y}{1} = \{\CPLock{n}, \CPThread{T3}, \CPThread{$\xi$}\},\\
&&&& \PCPLockSet{m}{1} = \{\PCPLock{o}{m}{1}, \CCPLock{n}{m}{1}, \PCPThread{T4}{m}{1}, \PCPThread{T3}{m}{1}\}, \CCPLockSet{y}{1} = \CCPLockSet{n}{1} = \CCPLockSet{q}{1} = \CCPLockSet{q}{2} = \emptyset,\\
&&&& \PCPLockSet{z}{1} = \{\PCPLock{o}{m}{1}, \CCPLock{n}{m}{1}, \PCPThread{T4}{m}{1}, \PCPThread{T3}{m}{1}, \PCPThread{$\xi$}{m}{1}\},\\
&&\Release{m}{2}&& \HBLockSet{o}{1} = \HBLockSet{m}{2} = \{\HBLock{o}{1}, \HBLock{n}{2}, \HBLock{m}{2}, \HBThread{T3}, \HBThread{T4}\}, \HBLockSet{n}{2} = \{\HBLock{n}{2}, \HBLock{m}{2}, \HBThread{T3}\}, \HBLockSet{y}{1} = \{\LSLock{n}{1}, \HBLock{m}{2}, \HBThread{T2}, \HBThread{T3}, \HBThreadPlain{\xi}\},\\
&&&& \HBLockSet{q}{1} = \{\HBLock{q}{1}, \HBLock{n}{1}, \HBLock{m}{2}, \HBThread{T1}, \HBThread{T2}, \HBThread{T3}\}, \HBLockSet{q}{2} = \{\HBLock{q}{2}, \HBLock{n}{1}, \HBLock{m}{2}, \HBThread{T2}, \HBThread{T3}\}, \HBLockSet{n}{1} = \{\HBLock{n}{1}, \HBLock{m}{2}, \HBThread{T2}, \HBThread{T3}\},\\
&&&& \CPLockSet{n}{1} = \CPLockSet{q}{1} = \CPLockSet{q}{2} = \{\CPLock{n}, \CPLock{m}, \CPThread{T3}\}, \CPLockSet{y}{1} = \{\CPLock{n}, \CPLock{m}, \CPThread{T3}, \CPThread{$\xi$}\},\\
&&&& \CPLockSet{m}{1} = \{\CPLock{n}, \CPLock{o}, \CPLock{m}, \CPThread{T3}, \CPThread{T4}\}, \CPLockSet{z}{1} = \{\CPLock{n}, \CPLock{o}, \CPLock{m}, \CPThread{T3}, \CPThread{T4}, \CPThread{$\xi$}\}, \CCPLockSet{z}{1} = \CCPLockSet{m}{1} = \emptyset

\end{tabular}
\textlink{1}{2}{\CP}
\caption{Example execution and \goldCP's analysis state.
In this execution, \CPOrdered{\Write{z}{1}}{\Write{z}{2}} because of a \CP ordering
that has not yet been established when \Write{z}{2} executes.}
\label{fig:tricky-true-ruleb}
\end{figure}

Figures~\ref{fig:tricky-true-ruleb} and \ref{fig:tricky-false-ruleb} show how a subtle change in
an execution can drastically affect the ordering between events.

In Figure~\ref{fig:tricky-true-ruleb},
\CPOrdered{\Write{z}{1}}{\Write{z}{2}} by the following logic:
\CPOrdered{\Release{n}{1}}{\Acquire{n}{2}} by \RuleA implies
\CPOrdered{\Acquire{m}{1}}{\Release{m}{2}} by \RuleC implies
\CPOrdered{\Release{m}{1}}{\Acquire{m}{2}} by \RuleB.
However, these \CP orderings are not knowable at \Write{z}{2}.
At \Write{z}{2}, \goldCP adds \PCPThreadPlain{\xi}{m}{1} to \PCPLockSet{z}{1},
since \CPOrdered{\Write{z}{1}}{\Write{z}{2}} if \CPOrdered{\Acquire{m}{1}}{\Release{m}{2}}.
As a result, at \Release{m}{2},
\raptor adds \CPThreadPlain{\xi} to \CPLockSet{z}{1} because $\CPThread{T3} \in \CPLockSet{m}{1}$.

% which is because $\Release{m}{1} \totalOrder
% \Acquire{q}{1}$. By tracking the \CP relation through lock instance
% \OwnerElement{m}{1}, the necessary total ordering from \Release{m}{1} to
% \Acquire{q}{1} is known and correctly establishes the \CP relation from
% \Release{m}{1} to \Acquire{m}{2}. The examples in
% Figure~\ref{fig:tricky-true-ruleb} and \ref{fig:tricky-false-ruleb} show case
% the need to track locksets for both lock instances and variable instances.

% \paragraph{Example that is subtly different from the prior example.}

\begin{figure}
\smaller
\centering

\newcolumntype{L}{>{$}l<{$}} % math-mode version of "l" column type

\begin{tabular}{@{}l@{\;}l@{\;\;}l@{\;}l@{\;}|L@{}}
\thr{T1} & \thr{T2} & \thr{T3} & \thr{T4} & \text{Updated analysis state after event (excluding \POLockSetPlain{\rho}{})}\\\hline
\Write{z}{1}&&&& \HBLockSet{z}{1} = \{\HBThread{T1}\}\\
\Acquire{q}{1}&&&& \HBLockSet{q}{1} = \{\HBThread{T1}\}\\
\Release{q}{1}&&&& \HBLockSet{z}{1} = \HBLockSet{q}{1} = \{\HBLock{q}{1}, \HBThread{T1}\}\\
\Acquire{m}{1}&&&& \HBLockSet{m}{1} = \{\HBThread{T1}\}\\
\Release{m}{1}&&&& \HBLockSet{m}{1} = \{\HBLock{m}{1}, \HBThread{T1}\}, \HBLockSet{z}{1} = \HBLockSet{q}{1} = \{\HBLock{q}{1}, \HBLock{m}{1}, \HBThread{T1}\}\\
&\Acquire{q}{2}&&& \HBLockSet{q}{2} = \{\HBThread{T2}\}, \HBLockSet{z}{1} = \HBLockSet{q}{1} = \{\HBLock{q}{1}, \HBLock{m}{1}, \HBThread{T1}, \HBThread{T2}\}, \PCPLockSet{z}{1} = \PCPLockSet{q}{1} = \{\PCPThread{T2}{q}{1}\}\\
&\Release{q}{2}&&& \HBLockSet{q}{2} = \{\HBLock{q}{2}, \HBThread{T2}\}, \CCPLockSet{z}{1} = \CCPLockSet{q}{1} = \emptyset\\
&\Acquire{n}{1}&&& \HBLockSet{n}{1} = \{\HBThread{T2}\}\\
&\Write{y}{1}&&& \HBLockSet{y}{1} = \{\LSLock{n}{1}, \HBThread{T2}\}\\
&\Release{n}{1}\tikzmark{1}&&& \HBLockSet{n}{1} = \{\HBLock{n}{1}, \HBThread{T2}\}, \HBLockSet{q}{2} = \{\HBLock{q}{2}, \HBLock{n}{1}, \HBThread{T2}\}, \HBLockSet{z}{1} = \HBLockSet{q}{1} = \{\HBLock{q}{1}, \HBLock{m}{1}, \HBLock{n}{1}, \HBThread{T1}, \HBThread{T2}\}\\
&&\Acquire{m}{2}&& \HBLockSet{z}{1} = \HBLockSet{q}{1} = \{\HBLock{q}{1}, \HBLock{m}{1}, \HBLock{n}{1}, \HBThread{T1}, \HBThread{T2}, \HBThread{T3}\}, \HBLockSet{m}{1} = \{\HBLock{m}{1}, \HBThread{T1}, \HBThread{T3}\}, \HBLockSet{m}{2} = \{\HBThread{T3}\},\\
&&&& \PCPLockSet{z}{1} = \PCPLockSet{q}{1} = \PCPLockSet{m}{1} = \{\PCPThread{T3}{m}{1}\}\\
&&\Acquire{o}{1}&& \HBLockSet{o}{1} = \{\HBThread{T3}\}\\
&&\Release{o}{1}&& \HBLockSet{z}{1} = \HBLockSet{q}{1} = \{\HBLock{q}{1}, \HBLock{m}{1}, \HBLock{n}{1}, \HBLock{o}{1}, \HBThread{T1}, \HBThread{T2}, \HBThread{T3}\}, \HBLockSet{m}{1} = \{\HBLock{m}{1}, \HBLock{o}{1}, \HBThread{T1}, \HBThread{T3}\},\\
&&&& \HBLockSet{o}{1} = \HBLockSet{m}{2} = \{\HBLock{o}{1}, \HBThread{T3}\}, \PCPLockSet{z}{1} = \PCPLockSet{q}{1} = \PCPLockSet{m}{1} = \{\PCPLock{o}{m}{1}, \PCPThread{T3}{m}{1}\}\\
&&&\Acquire{o}{2}& \HBLockSet{z}{1} = \HBLockSet{q}{1} = \{\HBLock{q}{1}, \HBLock{m}{1}, \HBLock{n}{1}, \HBLock{o}{1}, \HBThread{T1}, \HBThread{T2}, \HBThread{T3}, \HBThread{T4}\}, \HBLockSet{m}{1} = \{\HBLock{m}{1}, \HBLock{o}{1}, \HBThread{T1}, \HBThread{T3}, \HBThread{T4}\},\\
&&&& \HBLockSet{o}{1} = \HBLockSet{m}{2} = \{\HBLock{o}{1}, \HBThread{T3}, \HBThread{T4}\}, \HBLockSet{o}{2} = \{\HBThread{T4}\}, \PCPLockSet{o}{1} = \PCPLockSet{m}{2} = \{\PCPThread{T4}{o}{1}\},\\
&&&& \PCPLockSet{z}{1} = \PCPLockSet{q}{1} = \PCPLockSet{m}{1} = \{\PCPLock{o}{m}{1}, \PCPThread{T3}{m}{1}, \PCPThread{T4}{m}{1}, \PCPThread{T4}{o}{1}\}\\ 
&&&\Release{o}{2}& \HBLockSet{o}{2} = \{\HBLock{o}{2}, \HBThread{T4}\}, \PCPLockSet{z}{1} = \PCPLockSet{q}{1} = \PCPLockSet{m}{1} = \{\PCPLock{o}{m}{1}, \PCPThread{T3}{m}{1}, \PCPThread{T4}{m}{1}\},\\
&&&& \CCPLockSet{o}{1} = \CCPLockSet{m}{2} = \emptyset\\
&&&\Write{z}{2}& \HBLockSet{z}{1} = \{\HBLock{q}{1}, \HBLock{m}{1}, \HBLock{n}{1}, \HBLock{o}{1}, \HBThread{T1}, \HBThread{T2}, \HBThread{T3}, \HBThread{T4}, \HBThreadPlain{\xi}\}, \HBLockSet{z}{2} = \{\HBThread{T4}\},\\
&&&& \PCPLockSet{z}{1} = \{\PCPLock{o}{m}{1}, \PCPThread{T3}{m}{1}, \PCPThread{T4}{m}{1}, \PCPThread{$\xi$}{m}{1}\}\\
&&\tikzmark{2}\Acquire{n}{2}&& \HBLockSet{y}{1} = \{\LSLock{n}{1}, \HBThread{T2}, \HBThread{T3}\}, \HBLockSet{n}{2} = \{\HBThread{T3}\}, \HBLockSet{n}{1} = \{\HBLock{n}{1}, \HBThread{T2}, \HBThread{T3}\}, \HBLockSet{q}{2} = \{\HBLock{q}{2}, \HBLock{n}{1}, \HBThread{T2}, \HBThread{T3}\}\\
&&&& \PCPLockSet{q}{2} = \PCPLockSet{y}{1} = \PCPLockSet{n}{1} = \{\PCPThread{T3}{n}{1}\}, \PCPLockSet{q}{1} = \{\PCPLock{o}{m}{1}, \PCPThread{T3}{m}{1}, \PCPThread{T4}{m}{1}, \PCPThread{T3}{n}{1}\},\\
&&&& \PCPLockSet{z}{1} = \{\PCPLock{o}{m}{1}, \PCPThread{T3}{m}{1}, \PCPThread{T4}{m}{1}, \PCPThread{$\xi$}{m}{1}, \PCPThread{T3}{n}{1}\}\\
&&\Write{y}{2}&& \HBLockSet{y}{1} = \{\LSLock{n}{1}, \HBThread{T2}, \HBThread{T3}, \HBThreadPlain{\xi}\}, \HBLockSet{y}{2} = \{\LSLock{m}{2}, \LSLock{n}{2}, \HBThread{T3}\}, \CPLockSet{n}{1} = \{\CPThread{T3}\}, \PCPLockSet{y}{1} = \{\PCPThread{T3}{n}{1}, \PCPThread{$\xi$}{n}{1}\}\\
&&\Release{n}{2}&& \HBLockSet{m}{1} = \{\HBLock{m}{1}, \HBLock{o}{1}, \HBLock{n}{2}, \HBThread{T1}, \HBThread{T3}, \HBThread{T4}\}, \HBLockSet{o}{1} = \HBLockSet{m}{2} = \{\HBLock{o}{1}, \HBLock{n}{2}, \HBThread{T3}, \HBThread{T4}\}, \HBLockSet{n}{2} = \{\HBLock{n}{2}, \HBThread{T3}\}\\ 
&&&& \PCPLockSet{z}{1} = \{\PCPLock{o}{m}{1}, \CCPLock{n}{m}{1}, \PCPThread{T3}{m}{1}, \PCPThread{T4}{m}{1}, \PCPThread{$\xi$}{m}{1}\}, \CCPLockSet{q}{2} = \CCPLockSet{y}{1} = \CCPLockSet{n}{1} = \emptyset,\\
&&&& \PCPLockSet{q}{1} = \CCPLockSet{m}{1} = \{\PCPLock{o}{m}{1}, \CCPLock{n}{m}{1}, \PCPThread{T3}{m}{1}, \PCPThread{T4}{m}{1}\},\\
&&&& \CPLockSet{z}{1} = \CPLockSet{q}{1} = \CPLockSet{q}{2} = \CPLockSet{n}{1} = \{\CPLock{n}, \CPThread{T3}\}, \CPLockSet{y}{1} = \{\CPLock{n}, \CPThread{T3}, \CPThread{$\xi$}\}\\
&&\Release{m}{2}&& \HBLockSet{n}{2} = \{\HBLock{n}{2}, \HBLock{m}{2}, \HBThread{T3}\}, \HBLockSet{o}{1} = \HBLockSet{m}{2} = \{\HBLock{o}{1}, \HBLock{n}{2}, \HBLock{m}{2}, \HBThread{T3}, \HBThread{T4}\},\\
&&&& \HBLockSet{q}{2} = \{\HBLock{q}{2}, \HBLock{m}{2}, \HBLock{n}{1}, \HBThread{T2}, \HBThread{T3}\}, \HBLockSet{n}{1} = \{\HBLock{n}{1}, \HBLock{m}{2}, \HBThread{T2}, \HBThread{T3}\}, \HBLockSet{y}{1} = \{\LSLock{n}{1}, \HBLock{m}{2}, \HBThread{T2}, \HBThread{T3}, \HBThreadPlain{\xi}\},\\
&&&& \CPLockSet{z}{1} = \CPLockSet{q}{1} = \CPLockSet{q}{2} = \CPLockSet{n}{1} = \{\CPLock{n}, \CPLock{m}, \CPThread{T3}\}, \CPLockSet{y}{1} = \{\CPLock{n}, \CPLock{m}, \CPThread{T3}, \CPThread{$\xi$}\},\\
&&&& \CCPLockSet{z}{1} = \CCPLockSet{q}{1} = \emptyset

\end{tabular}
\textlink{1}{2}{\CP}
\caption{Example execution and \goldCP's analysis state.
This example is subtlely different from the example in Figure~\ref{fig:tricky-true-ruleb}:
it flips the order of \thr{T1}'s critical sections on \code{m} and \code{q}.
As a result, \protect\NotCPOrdered{\Acquire{m}{1}}{\Release{m}{2}} and \protect\NotCPOrdered{\Write{z}{1}}{\Write{z}{2}}.}
\label{fig:tricky-false-ruleb}
\end{figure}

Figure~\ref{fig:tricky-false-ruleb} differs from
Figure~\ref{fig:tricky-true-ruleb} only by changing the order in which
\thr{T1} executes its critical sections on \code{m} and \code{q}.
This subtle change means that \NotCPOrdered{\Release{m}{1}}{\Acquire{m}{2}}, which
results in \NotCPOrdered{\Write{z}{1}}{\Write{z}{2}}.

In Figure~\ref{fig:tricky-false-ruleb},
directly after \Release{q}{1}, $\HBLock{m}{1} \in \HBLockSet{q}{1}$,
instead of $\HBLock{q}{1} \in \HBLockSet{m}{1}$ as in Figure~\ref{fig:tricky-true-ruleb}.
As a result, $\PCPThread{T3}{n}{1} \notin \PCPLockSet{m}{1}$ after \Acquire{n}{2}.
That is, \goldCP correctly captures that, in this example,
\CPOrdered{\Acquire{n}{1}}{\Release{n}{2}} does \emph{not} imply
\CPOrdered{\Acquire{m}{1}}{\Release{m}{2}}.

% In Figure~\ref{fig:tricky-false-ruleb}
% \Ordered{\Write{z}{1}}{\centernot{\CPRelation}}{\Write{z}{2}} because
% \Ordered{\Release{m}{1}}{\centernot{\CPRelation}}{\Acquire{m}{2}} because
% $\Release{q}{1} \totalOrder \Acquire{m}{1}$. This example is tricky since
% \OwnerElement{z}{1} locksets will establish \CP relation to \thr{T4} if
% \HBLock{m}{1} has a \CP relation to \thr{T3} at \Release{m}{2}. 

% By tracking the \CP relation from \Acquire{m}{1} to \Release{m}{2} through
% \OwnerElement{m}{1} lockset it is possible to distinguish when \Acquire{m}{1}
% event occurred with respect to \Release{q}{1}. By tracking the \CP relation for
% both variables and locks less information about the ordering of events is needed
% per lockset.
% Otherwise, \OwnerElement{z}{1} would have had to keep track of not only which
% lock elements, but also the order they occurred in.

\subsection{A More Complex Example Showing the Need for Transferring Ordering}
% \paragraph{More complex example showing the need for transferring ordering.}

\jake{I don't think this example is needed considering Figure 6 already
exists. The same point is being made about transferring CCP order just using a
different trace. If the suggestion for the prior two appendix examples is not
well received then I would suggest using this example as the subtle difference
to Figure 6. It handles the concept of the subtle difference while reinforcing
the CCP transfer concept with a complex example.
\mike{So assuming we're not going to change Figures 2 or 5,
are you suggesting keeping this example in the appendix and removing the other appendix examples?
Or something else? You don't think Figure 8 is showing anything particularly unique/special (I don't have much of an opinion
without diving deeply into \raptor again)?}}

\input{examples/ComplexExample}

Figure~\ref{fig:ComplexExample} shows an example that involves transfer of \PCP ordering but that
is more complex than Section~\ref{sec:analysis}'s Figure~\ref{fig:ruleb-transfer-needed}.
% Figure~\ref{fig:ComplexExample} illustrates some of the challenges involved in developing an online
% analysis for \CP.
In this example,
the writes to \code{x} are \CP ordered because the critical sections on \code{m} are \CP ordered, which is true
because the critical sections on \code{n} are \CP ordered.
More precisely,
\CPOrdered{\Write{x}{1}}{\Write{x}{2}} by the following logic:
\CPOrdered{\Release{n}{1}}{\Acquire{n}{2}} by \RuleA implies
\CPOrdered{\Acquire{m}{1}}{\Release{m}{2}} by \RuleC implies
\CPOrdered{\Release{m}{1}}{\Acquire{m}{2}} by \RuleB implies
\CPOrdered{\Write{x}{1}}{\Write{x}{2}} by \RuleC.

However, at the event \Release{m}{2},
an online analysis \emph{cannot} determine that
\CPOrdered{\Acquire{m}{1}}{\Release{m}{2}} (and thus \CPOrdered{\Release{m}{1}}{\Acquire{m}{2}})
because it is \emph{not knowable} that 
\CPOrdered{\Release{n}{1}}{\Acquire{n}{2}}.

Furthermore, at \Write{x}{2}, an online analysis \emph{cannot} determine that
\CPOrdered{\Write{x}{1}}{\Write{x}{2}} because it is not knowable that
\CPOrdered{\Release{m}{1}}{\Acquire{m}{2}} or \CPOrdered{\Release{n}{1}}{\Acquire{n}{2}}.
Not until \Write{y}{2} is it knowable
that \CPOrdered{\Release{n}{1}}{\Acquire{n}{2}} and thus
\CPOrdered{\Release{m}{1}}{\Acquire{m}{2}} and thus
\CPOrdered{\Write{x}{1}}{\Write{x}{2}}.

At \Release{m}{2},
\goldCP transfers \PCP ordering from \code{m} to \code{n} by adding
\PCPThread{T5}{n}{1} to \PCPLockSet{x}{1} because
$\PCPThread{T4}{n}{1} \in \PCPLockSet{m}{1}$ and
$\PCPThread{T5}{m}{1} \in \PCPLockSet{x}{1}$.
At \Write{x}{2}, the analysis thus adds \PCPThreadPlain{\xi}{n}{1} to \PCPLockSet{x}{1}.
Finally, at \Release{n}{2}, \goldCP adds $\xi$ to \CPLockSet{x}{1} because $\CPThread{T3} \in \CPLockSet{n}{1}$.

\notes{
Now suppose instead that \thr{T1} executed its critical section on \code{t}
\emph{before} its critical section on \code{m}.
In that subtly different execution, \NotCPOrdered{\Write{x}{1}}{\Write{x}{2}}.
A sound and complete online analysis for \CP must track analysis state
that captures the difference between these two different cases.
}
